# Supplementary material for: Epidemiology-Aware Neural ODE with Continuous Disease Transmission Graph
Source: arXiv:2410.00049 source file (2024-11-10)
Supplement: Supplementary file 1 [file appendix.tex]

% \paragraph{Roadmap of Appendix} The Appendix is organized as follows.
% We list the notations table in Section~\ref{app:notation}.
% We provide theoretical proof of convergence in Section~\ref{app:proof}. 
% The algorithm of FedBN is described in Section~\ref{app:algorithm}.
\section{Appendix}

\section{Notation Table}
\label{app:notation}		
\begin{table}[h]\small
\centering
\scriptsize{\resizebox{0.9\linewidth}{!}{
\begin{tabular}{cl}
\hline
Notations & Description \\ \hline
%base
$A$ & adjacency matrix \\
$Y$ & labels of graph \\
$X$ & node featurs \\
$v_i$ & the node with indicator $i$ in graph \\
$y_i$ & label of node $v_i$\\
$A_i$ & the neighborhoods of the node $v_i$ \\
$Z$ & node-level feature, $\text{hidden dimension} \in \mathbb{R}^d$ \\ 
$U$ & output logit \\
$d$ & dimension of $z$ \\
$I$ & classes collection \\
$f$ & feature extractor \\
$g$ & classifier head \\

%method
$\mathcal{B}$ & global memory bank \\
$k$ & k-nearest neighbors in FCPP \\
$k'$ & k-nearest neighbors in global semantic graph completion \\
$c$ & prototype \\
$j$ & the index of class \\
$\omega( \cdot )$ & cosine similarity \\
$\mathbb{C}^j$ & prototypes collections \\
$w_i$ & node weight in prototype aggregation \\
$W$ & the weight sum \\
$H$ & cluster centroids num \\
$\mathbf{G}$ & the graph augmentation module \\
$F$ & hidden features in GKIC \\
$g$ & the global signal \\
$\Omega$ & probability matrix \\
$\lambda$ & the strength of augmentation \\
$\mathbf{S}$ & a Gumbel random variate \\
$\mathbb{H}$ & cross-entropy loss \\

%fed
$M$ & total number of clients \\
$m$ & the index of client \\
$P$ & distribution \\
$D^m$ & private data of the  $m$ client\\
$R$ & communication round \\
$\theta^m$ & model parameter of client $m$ \\
$E$ & local training epochs \\
% $\sigma(\cdot)$ & ReLU activation function, $\sigma(\cdot) = \max\{\cdot,0\}$ \\
$\tau$ & the parameter in contrastive method \\
$\alpha$ & the loss weight for $L_{con}$\\
$\beta$ & the loss weight for $L_{reg}$ \\
$\eta$ & learning rate  \\
\hline
\end{tabular}%
}}

\caption{Notations occurred in the paper.}
\label{tab:notation}
\end{table}
